# Supplementary material for: Revealing and Mitigating Over-Attention in Knowledge Editing
Source: arXiv:2502.14838 source file (2025-02-20)
Supplement: Supplementary file 1 [file main_exp_appendix.tex]

\addtolength{\tabcolsep}{2pt}

\begin{table*}[!htbp]
    \centering
    \tiny
    \caption{Results of our methods on...}
    \label{tab:main}
    \begin{adjustbox}{width=1\textwidth}
    \begin{tabular}{ccrrrrrrrrrrrr}
    \toprule
         \multicolumn{1}{c}{\textbf{Model}}&\multicolumn{1}{c}{\textbf{Editor}} & \multicolumn{2}{c}{\textbf{Rewrite}} & \multicolumn{2}{c}{\textbf{Generalization}} & \multicolumn{7}{c}{\textbf{Specificity}} & \multicolumn{1}{c}{\textbf{Fluency}} \\
        \cmidrule(lr){3-4}\cmidrule(lr){5-6}\cmidrule(lr){7-13}\cmidrule(lr){14-14}
        && ES $\uparrow$ & EM $\uparrow$ & PS $\uparrow$ & PM $\uparrow$ & NS $\uparrow$ & NM $\uparrow$ & RS $\uparrow$ & RM $\uparrow$ & NES $\uparrow$ & NEM $\uparrow$ & GES $\uparrow$ & FL $\uparrow$\\
        \midrule
    \multirow{8}{*}{GPT2-XL} 
    &None&21.99& 0.52 & 23.48&0.35 & 77.37 &4.60 & 76.35 &6.38 & 49.87& 10.86 & 5.43 & 6.26  \\
    \cmidrule(lr){2-14}
    &ROME& \bf 99.46 & \bf 92.90 & \bf 96.90 & \bf 61.20 & 75.74&\bf 4.68 & 23.01 &2.95 & 13.63 & 5.22 & 4.15 & 6.23    \\
    &+ ours& 99.34 & 85.18 & 93.56 & 45.46 & \bf 76.13 & 4.65 & \bf 24.85 & \bf 4.71 & \bf 20.88 & \bf 7.71 & \bf 5.32 & 6.23 \\
    \cmidrule(lr){2-14}
    & MEMIT \\
    & +ours \\
    \cmidrule(lr){2-14}
    & PEMT \\
    & +ours \\
    \cmidrule(lr){1-14}
    \multirow{8}{*}{GPT-J} 
    &None&20.86&0.64 & 17.70&0.40 &82.00 &6.32 & 79.79&8.69 & 62.65& 14.21 & 7.38 & 6.22  \\
    \cmidrule(lr){2-14}
    &ROME& \bf99.88 & \bf99.39 & \bf99.58 & \bf76.93& 79.45&6.13 & 11.14&3.19 & 30.13& 10.51 &7.05 & 6.21  \\
    &+ ours&99.76&98.37 & 95.35& 53.95& \bf80.55& \bf6.27& \bf26.48& \bf6.83& \bf47.13& \bf14.34 &\bf7.38 & 6.21  \\
    \cmidrule(lr){2-14}
    & MEMIT \\
    & +ours \\
    \cmidrule(lr){2-14}
    & PEMT \\
    & +ours \\
    \cmidrule(lr){1-14}
    \multirow{8}{*}{Llama2-7b} 
    &None  \\
    \cmidrule(lr){2-14}
    &ROME  \\
    &+ ours  \\
    \cmidrule(lr){2-14}
    & MEMIT \\
    & +ours \\
    \cmidrule(lr){2-14}
    & PEMT \\
    & +ours \\
    \bottomrule
    \end{tabular}
    \end{adjustbox}
\end{table*}%

\addtolength{\tabcolsep}{-2pt}
